# Supplementary material for: A Simulation-free Group Sequential Design with Max-combo Tests in the Presence of Non-proportional Hazards
Source: arXiv:1911.05684 source file (2023-01-17)
Supplement: Supplementary file 1 [file supprt_inf.tex]

\documentclass[12pt]{article}
\usepackage{amssymb,amsmath,bm,amsthm}
\usepackage{amsfonts}
\usepackage{graphicx}
\usepackage{listings}
\usepackage{geometry}
\usepackage{setspace}
\usepackage{caption}
\usepackage{lscape}
\theoremstyle{remark}

\captionsetup[table]{name=Web Table}
\captionsetup[figure]{name=Wab Figure}
\doublespacing
\title{Supporting information for (A Simulation-free Group Sequential Design with Max-combo Tests in the Presence of Non-proportional Hazards) by (Lili Wang, Xiaodong Luo, and Cheng Zheng)}
\author{}
\date{}
%As discussed in detail below, supplementary web material may include some or all of: additional written exposition, tables, and figures. All such supplementary material should be placed in a single document entitled "Web-based Supplementary Materials for (title of manuscript) by (authors)."  followed by "Web Table 1," "Web Table 2," etc. for supplementary tables; and "Web Figure 1," etc., for supplementary figures. Web Tables and Figures should have descriptive captions in the same style as those for tables and figures included in a main manuscript. Web Appendices, Tables, and Figures may be referenced in the main manuscript as, for example, "See Web Appendix A for the derivation of Equation (1)" or "Web Tables 1-4 present results of additional simulations."
\begin{document}
\maketitle

\section{Web Appendix A: violation of event hazards} \label{A1}
In addition to the violations of both censoring and accrual procedures (Table~2), we also let the event hazard $\lambda$ be misspecified. Let the actual median survival time be 12 months instead of 6 months, indicating that the hazard is $\lambda=\log(2)/12$. According to Web Table~\ref{tab:violation2}, the type I error did not change, while the power was much larger than $0.9$. A plausible explanation could be the stopping times were higher than those with $\lambda=\log(2)/6$, and thus more events during were observed the late departure period, ending up with power higher than the nominal $0.9$. In contrast, when the hazard is higher than $\lambda=\log(2)/6$, one would expect that the power would be less than the nominal $0.9$. 
 %%%% Supplemental table 1  %%%%
%\begin{sidewaystable}
\begin{table}[h!]
\begin{minipage}{160mm}\centering
\caption{The rejection probabilities under the null hypothesis denoted by $H_0$ (type I error) and under the alternative hypothesis $H_1$ (power) \emph{ when the censoring, accrual and event hazards are misspecified}. Prefixes ``GS''  standing for ``group-sequential'' are eliminated here for simplicity.  }
\label{tab:violation2}
\begin{tabular}{lllcclcclccl}\hline\hline
\phantom{}&{}&\phantom{}&\multicolumn{2}{c}{ $\theta=0.7$} &
&\multicolumn{2}{c}{ $\theta=0.6$} &\phantom{}&\multicolumn{2}{c}{ $\theta=0.5$} &\phantom{}\\ [-1pt]
\cline{4-5} \cline{7-8} \cline{10-11}\\[-10pt]
 &Test&Stage&$H_0$&$H_1$& &$H_0$&$H_1$& & $H_0$&$H_1$& \\ \hline
&WLRT& combined           &0.0264&0.9536& &0.0263&0.9555& &0.0261&0.9575&\\
&    & interim            &0.0051&0.5108& &0.0052&0.5172& &0.0048&0.5138&\\
&SLRT& combined           &0.0250&0.9449& &0.0245&0.9438& &0.0243&0.9434&\\
&    & interim            &0.0051&0.4331& &0.0051&0.4265& &0.0049&0.4164&\\
&MC (naive)&combined      &0.0380&0.9703& &0.0376&0.9707& &0.0376&0.9723&\\
&    & interim            &0.0083&0.5675& &0.0083&0.5695& &0.0079&0.5644&\\
&MC (pred-sto)&combined   &0.0245&0.9551& &0.0242&0.9561& &0.0244&0.9573&\\
&    &interim             &0.0050&0.4992& &0.0052&0.5015& &0.0047&.4956&\\
&MC (pred-exa)&    combined &0.0246&0.9552& &0.0243&0.9562& &0.0244&0.9573&\\
&           &     interim  &0.0051&0.4995& &0.0052&0.5017& &0.0047&0.4959&\\
&MC (est)&    combined  &0.0245&0.9552& &0.0243&0.9561& &0.0244&0.9573&\\
&           &     interim &0.0051&0.5007& &0.0052&0.5029& &0.0047&0.4969&\\
\hline
\end{tabular}
\end{minipage}
\vspace{5pt}
\end{table}
%\end{sidewaystable}
%%%%  end Supplemental table 1  %%%%

\section{Web Appendix B: violation of delayed time} \label{A2}
In addition to the violations of both the censoring and the accrual were violated (as in Table~2), we also let the delayed time $\epsilon$ be misspecified, i.e., the actual change time is $\epsilon=6$ other than $\epsilon=2$. According to Web Table~\ref{tab:violation3}, the misspecifications did not affect the type I error computation, but largely reduced the power. The reason is that the expected treatment effect is much earlier than its exact starting time. Thus the sample size is underestimated. 

 %%%% Supplemental table 2  %%%%
%\begin{sidewaystable}
\begin{table}[h!]
\begin{minipage}{160mm}\centering
\caption{The rejection probabilities under the null hypothesis denoted by $H_0$ (type I error) and under the alternative hypothesis $H_1$ (power) \emph{ when the censoring, accrual and delayed time are misspecified}. Prefixes ``GS''  standing for ``group-sequential'' are eliminated here for simplicity.  }
\label{tab:violation3}
\begin{tabular}{lllcclcclccl}\hline\hline
\phantom{}&{}&\phantom{}&\multicolumn{2}{c}{ $\theta=0.7$} &
&\multicolumn{2}{c}{ $\theta=0.6$} &\phantom{}&\multicolumn{2}{c}{ $\theta=0.5$} &\phantom{}\\ [-1pt]
\cline{4-5} \cline{7-8} \cline{10-11}\\[-10pt]
 &Test&Stage&$H_0$&$H_1$& &$H_0$&$H_1$& & $H_0$&$H_1$& \\ \hline
&WLRT& combined           &0.0259&0.3805& &0.0261&0.3459& &0.0268&0.3136&\\
&    & interim            &0.0052&0.0279& &0.0053&0.0270& &0.0052&0.0230&\\
&SLRT& combined           &0.0248&0.1834& &0.0248&0.1634& &0.0250&0.1490&\\
&    & interim            &0.0053&0.0136& &0.0051&0.0129& &0.0051&0.0122&\\
&MC (naive)&combined      &0.0379&0.3923& &0.0383&0.3581& &0.0391&0.3261&\\
&    & interim            &0.0085&0.0330& &0.0084&0.0317& &0.0084&0.0276&\\
&MC (pred-sto)&combined   &0.0246&0.3215& &0.0247&0.2922& &0.0256&0.2627&\\
&    &interim             &0.0052&0.0218& &0.0052&0.0212& &0.0051&0.0183&\\
&MC (pred-exa)&    combined &0.0246&0.3219& &0.0248&0.2926& &0.0256&0.2629&\\
&           &     interim  &0.0053&0.0219& &0.0052&0.0212& &0.0051&0.0184&\\
&MC (est)&    combined  &0.0246&0.3224& &0.0247&0.2931& &0.0256&0.2635&\\
&           &     interim &0.0052&0.0218& &0.0051&0.0212& &0.0051&0.0183&\\
\hline
\end{tabular}
\end{minipage}
\vspace{5pt}
\end{table}
%\end{sidewaystable}
%%%%  end Supplemental table 2  %%%%

\section{Web Appendix C: correlation matrices}

 %%%% Supplemental table 3  %%%%
%\begin{sidewaystable}
\begin{table}
	\begin{minipage}{160mm}\centering
		\caption{Comparison of the correlations computed using different methods: the correlations calculated directly from the simulated samples ($\overline{cor}$), the predicted values using either stochastic process ($\widetilde{cor}_{sto}$) or exact distribution ($\widetilde{cor}_{exa}$), and the data-driven estimation ($\widehat{cor}$). The sample correlations were treated as the gold standard for comparison of other methods.  In comparison with the gold-standard mean, correlations with difference $5-10\%$ were made \textit{italic}, and $>10\%$ were made \textbf{bold}.  There are \emph{not any violations} in accrual (I), censoring (II), survival functions (III) or delayed time (IV).}
		\label{tab:corr_all}
		\begin{tabular}{clcclcclcc}\hline\hline
			{Correlation }&\phantom{}&\multicolumn{2}{c}{ $\theta=0.7$} &
			&\multicolumn{2}{c}{ $\theta=0.6$} &\phantom{}&\multicolumn{2}{c}{ $\theta=0.5$}\\ [-1pt]\cline{3-4} \cline{6-7} \cline{9-10}\\[-10pt]
			Pair& &$H_0$&$H_1$& &$H_0$&$H_1$& &$H_0$&$H_1$ \\ \hline
			$\mathcal{G}_{0,1}(t_{int})$&$\overline{cor} $&0.8327&0.8329& &0.8329&0.8348&	&0.8310 &0.8351\\			
			 \ \&$\mathcal{G}_{0,0}(t_{int})$& $\widetilde{cor}_{sto}-\overline{cor} $ &-0.0024&-0.0021&	&-0.0029&-0.0038& &-0.0012&-0.0038\\
			    & $\widetilde{cor}_{exa}-\overline{cor} $ &-0.0004&0.0001&	&-0.0009&-0.0015& &0.0008&-0.0014\\			
			    & $\widehat{cor}-\overline{cor} $ &-0.0009&-0.0005&	&-0.0017&-0.0027& &-0.0008&-0.0033\\
			
			$\mathcal{G}_{0,1}(t_{fin})$&$\overline{cor} $&0.8469&0.8521&	&0.8452&0.8516&	&0.8417&0.8511\\
			  \ $\&\mathcal{G}_{0,0}(t_{fin})$  & $\widetilde{cor}_{sto}-\overline{cor} $ &0.0129&0.0167&	&0.0107&0.0145&	&0.0100&0.0139\\
			    & $\widetilde{cor}_{exa}-\overline{cor} $ &0.0142&0.0182&	&0.0120&0.0162&	&0.0114&0.0159\\
			    & $\widehat{cor}-\overline{cor} $ &-0.0001&-0.0015&	&-0.0010&-0.0018&	&0.0002&-0.0019\\
			
			$\mathcal{G}_{0,0}(t_{int})$&$\overline{cor} $&0.7754&0.7776& &0.7766&0.7791& &0.7751&0.7807\\
			 \  $\&\mathcal{G}_{0,0}(t_{fin})$ & $\widetilde{cor}_{sto}-\overline{cor} $ &-0.0020&-0.0036&	&-0.0037&-0.0033&	&0.0008&-0.0021\\
			    & $\widetilde{cor}_{exa}-\overline{cor} $ &0.0025&-0.0008& &-0.0046&-0.0016& &0.0000&-0.0067\\
			    & $\widehat{cor}-\overline{cor} $ &-0.0008&-0.0030&	&-0.0020&-0.0045&	&-0.0005&-0.0061\\
			
			$\mathcal{G}_{0,1}(t_{int})$&$\overline{cor} $&0.6399&0.6213&	&0.6457&0.6267&	&0.6459&0.6243\\
			    \ $\&\mathcal{G}_{0,1}(t_{fin})$& $\widetilde{cor}_{sto}-\overline{cor} $ &-0.0040&-0.0032&	&-0.0068&-0.0074&	&0.0015&-0.0019\\
			    & $\widetilde{cor}_{exa}-\overline{cor} $ &0.0034&0.0011&	&-0.0068&-0.0052&	&0.0015&-0.0091\\ 
			    & $\widehat{cor}-\overline{cor} $ &-0.0007&-0.0013&	&-0.0012&-0.0077&	&0.0014&-0.0085\\
			
			$\mathcal{G}_{0,1}(t_{int})$&$\overline{cor} $&0.6453&0.6444&	&0.6475&0.6493&	&0.6440&0.6473\\ 
		   \ $\&\mathcal{G}_{0,0}(t_{fin})$ & $\widetilde{cor}_{sto}-\overline{cor} $ &-0.0031&-0.0015& &-0.0060&-0.0046&	&-0.0002&-0.0001\\
			   & $\widetilde{cor}_{exa}-\overline{cor} $ &0.0022&0.0025&	&-0.0052&-0.0014&	&0.0006&-0.0021\\
			    & $\widehat{cor}-\overline{cor} $ &-0.0009&0.0003&	&-0.0037&-0.0047& &-0.0009&-0.0030\\             
			
			$\mathcal{G}_{0,0}(t_{int})$&$\overline{cor} $&0.5325&0.5228&	&0.5375&0.5262& &0.5364&0.5273\\
			    \ $\&\mathcal{G}_{0,1}(t_{fin})$& $\widetilde{cor}_{sto}-\overline{cor} $ &-0.0046&-0.0093&	&-0.0071&-0.0115&	&0.0009&-0.0098\\
			    & $\widetilde{cor}_{exa}-\overline{cor} $ &0.0029&-0.0044&	&-0.0059&-0.0083&	&0.0021&-0.0144\\
			    & $\widehat{cor}-\overline{cor} $ &-0.0008&-0.0068& &-0.0018&-0.0111&	&0.0010&-0.0151\\
			\hline
		\end{tabular}
	\end{minipage}
	\vspace{5pt}
\end{table}
%\end{sidewaystable}
%%%%  end Supplemental table 3  %%%%

 %%%% Supplemental table 4  %%%%
%\begin{sidewaystable}
\begin{table}
	\begin{minipage}{160mm}\centering
		\caption{Comparison of the correlations computed using different methods: the correlations calculated directly from the simulated samples ($\overline{cor}$), the predicted values using either stochastic process ($\widetilde{cor}_{sto}$) or exact distribution ($\widetilde{cor}_{exa}$), and the data-driven estimation ($\widehat{cor}$). The sample correlations were treated as the gold standard for comparison of other methods. In comparison with the gold-standard mean, correlations with difference $5-10\%$ were made \textit{italic}, and $>10\%$ were made \textbf{bold}. The simulations in this table include \emph{violations I (accrual) and II (censoring)}.  }
		\label{tab:corr_all1}
		\begin{tabular}{clcclcclcc}\hline\hline
	{Correlation }&\phantom{}&\multicolumn{2}{c}{ $\theta=0.7$} &
	&\multicolumn{2}{c}{ $\theta=0.6$} &\phantom{}&\multicolumn{2}{c}{ $\theta=0.5$}\\ [-1pt]\cline{3-4} \cline{6-7} \cline{9-10}\\[-10pt]
	Pair& &$H_0$&$H_1$& &$H_0$&$H_1$& &$H_0$&$H_1$ \\ \hline
			$\mathcal{G}_{0,1}(t_{int})$&$\overline{cor} $&0.8267&0.8304&	&0.8261&0.8263&	&0.8248&0.8295\\			
			    \ \&$\mathcal{G}_{0,0}(t_{int})$& $\widetilde{cor}_{sto}-\overline{cor} $ &0.0036&0.0004&	&0.0040&0.0047&	&0.0051&0.0018\\						
			    & $\widetilde{cor}_{exa}-\overline{cor} $ &0.0056&0.0026&	&0.0059&0.0070&	&0.0070&0.0042\\						
			    & $\widehat{cor}-\overline{cor} $ &-0.0009&-0.0036&	&-0.0007&0.0006&	&-0.0001&-0.0024\\
			
			$\mathcal{G}_{0,1}(t_{fin})$&$\overline{cor} $&0.8508&0.8539&	&0.8482&0.8529&	&0.8452&0.8522\\						
			   \ \&$\mathcal{G}_{0,0}(t_{fin})$& $\widetilde{cor}_{sto}-\overline{cor} $ &0.0189&0.0192&	&0.0176&0.0230&	&0.0163&0.0196\\						
			    & $\widetilde{cor}_{exa}-\overline{cor} $ &0.0201&0.0207&	&0.0188&0.0247&	&0.0176&0.0215\\
			    & $\widehat{cor}-\overline{cor} $ &-0.0010&-0.0015&	&-0.0008&-0.0014&	&-0.0002&-0.0016\\
			
			$\mathcal{G}_{0,0}(t_{int})$&$\overline{cor} $&0.7772&0.7789&	&0.7763&0.7797&	&0.7757&0.7824\\			
			  \ \&$\mathcal{G}_{0,0}(t_{fin})$& $\widetilde{cor}_{sto}-\overline{cor} $ &-0.0039&-0.0050&	&-0.0035&-0.0039&	&0.0002&-0.0038\\
			    & $\widetilde{cor}_{exa}-\overline{cor} $ &0.0006&-0.0022&	&-0.0043&-0.0021&	&-0.0007&-0.0085\\			
			    & $\widehat{cor}-\overline{cor} $ &-0.0027&-0.0043&	&-0.0017&-0.0051&	&-0.0011&-0.0078\\
			
			$\mathcal{G}_{0,1}(t_{int})$&$\overline{cor} $&0.6099&0.5826&	&0.6158&0.5884&	&0.6219&0.5864\\
			    \ \&$\mathcal{G}_{0,1}(t_{fin})$& $\widetilde{cor}_{sto}-\overline{cor} $ &0.0260&\textit{0.0355}&	&0.0232&\textit{0.0309}&	&0.0255&\textit{0.0361}\\			
			    & $\widetilde{cor}_{exa}-\overline{cor} $ &\textit{0.0334}&\textit{0.0398}&	&0.0232&\textit{0.0331}&	&0.0255&0.0288\\ 
			    & $\widehat{cor}-\overline{cor} $ &-0.0029&-0.0015&	&0.0000&-0.0082& &0.0005&-0.0092\\
			
			$\mathcal{G}_{0,1}(t_{int})$&$\overline{cor} $&0.6436&0.6456&	&0.6414&0.6454&	 &0.6413&0.6472\\ 
			    \ \&$\mathcal{G}_{0,0}(t_{fin})$& $\widetilde{cor}_{sto}-\overline{cor} $ &-0.0014&-0.0026& &0.0002&-0.0008&	&0.0025&0.0001\\
			    & $\widetilde{cor}_{exa}-\overline{cor} $ &0.0039&0.0014&	&0.0009&0.0024&	&0.0034&-0.0020\\
			    & $\widehat{cor}-\overline{cor} $ &-0.0038&-0.0052&	&-0.0020&-0.0049&	&-0.0025&-0.0065\\             
			
			$\mathcal{G}_{0,0}(t_{int})$&$\overline{cor} $&0.5044&0.4862&	&0.5093&0.4887&	&0.5117&0.4912\\
			    \ \&$\mathcal{G}_{0,1}(t_{fin})$& $\widetilde{cor}_{sto}-\overline{cor} $ &0.0236&\textit{0.0273}&	&0.0211&\textit{0.0260}&	&0.0255&\textit{0.0263}\\
			    & $\widetilde{cor}_{exa}-\overline{cor} $ &\textit{0.0311}&\textit{0.0322}&	&0.0223&\textit{0.0292}&	&\textit{0.0268}&0.0217\\
			    & $\widehat{cor}-\overline{cor} $ &-0.0031&-0.0059&	&-0.0011&-0.0089&	&0.0015&-0.0138\\
			\hline
		\end{tabular}
	\end{minipage}
	\vspace{5pt}
\end{table}
%\end{sidewaystable}
%%%%  end Supplemental table 4  %%%%

 %%%% Supplemental table 5  %%%%
%\begin{sidewaystable}
\begin{table}
	\begin{minipage}{160mm}\centering
		\caption{Comparison of the correlations computed using different methods: the correlations calculated directly from the simulated samples ($\overline{cor}$), the predicted values using either stochastic process ($\widetilde{cor}_{sto}$) or exact distribution ($\widetilde{cor}_{exa}$), and the data-driven estimation ($\widehat{cor}$). The sample correlations were treated as the gold standard for comparison of other methods. In comparison with the gold-standard mean, correlations with difference $5-10\%$ were made \textit{italic}, and $>10\%$ were made \textbf{bold}.  The simulations in this table include \emph{violations I (accrual), II (censoring), and III(event rate)}.  }
		\label{tab:corr_all2}
		\begin{tabular}{clcclcclcc}\hline\hline
	{Correlation }&\phantom{}&\multicolumn{2}{c}{ $\theta=0.7$} &
	&\multicolumn{2}{c}{ $\theta=0.6$} &\phantom{}&\multicolumn{2}{c}{ $\theta=0.5$}\\ [-1pt]\cline{3-4} \cline{6-7} \cline{9-10}\\[-10pt]
	Pair& &$H_0$&$H_1$& &$H_0$&$H_1$& &$H_0$&$H_1$ \\ \hline
			$\mathcal{G}_{0,1}(t_{int})$&$\overline{cor} $&0.8361&0.8429&	&0.8343&0.8409&	 &0.8306&0.8372\\						
			    \ \&$\mathcal{G}_{0,0}(t_{int})$& $\widetilde{cor}_{sto}-\overline{cor} $ &-0.0057&-0.0121&	&-0.0042&-0.0100&	&-0.0007&-0.0059\\						
			    & $\widetilde{cor}_{exa}-\overline{cor} $ &-0.0037&-0.0099&	&-0.0023&-0.0077&	&0.0012&-0.0035\\						
			    & $\widehat{cor}-\overline{cor} $ &-0.0004&-0.0022&	&-0.0008&-0.0004&	&0.0004&0.0029\\
					
			$\mathcal{G}_{0,1}(t_{fin})$&$\overline{cor} $&0.8548&0.8541&	&0.8540&0.8536& &0.8522&0.8516\\						
			   \ \&$\mathcal{G}_{0,0}(t_{fin})$& $\widetilde{cor}_{sto}-\overline{cor} $ &0.0096&0.0067&	&0.0094&0.0083&	&0.0105&0.0119\\						
			    & $\widetilde{cor}_{exa}-\overline{cor} $ &0.0108&0.0082&	&0.0106&0.0100&	&0.0118&0.0139\\
			    & $\widehat{cor}-\overline{cor} $ &-0.0007&-0.0009&	&-0.0006&-0.0014&	&0.0002&-0.0009\\
			
			$\mathcal{G}_{0,0}(t_{int})$&$\overline{cor} $&0.7771&0.7802&	&0.7777&0.7828&	&0.7767&0.7859\\			
			   \ \&$\mathcal{G}_{0,0}(t_{fin})$& $\widetilde{cor}_{sto}-\overline{cor} $ &-0.0037&-0.0063&	&-0.0048&-0.0070&	&-0.0008&-0.0073\\
			    & $\widetilde{cor}_{exa}-\overline{cor} $ &0.0008&-0.0035& &-0.0057&-0.0052&	&-0.0016&-0.0119\\			
			    & $\widehat{cor}-\overline{cor} $ &-0.0025&-0.0056&	&-0.0031&-0.0082&	&-0.0021&-0.0113\\
			
			$\mathcal{G}_{0,1}(t_{int})$&$\overline{cor} $&0.4978&0.4820&	&0.5047&0.4884&	 &0.5104&0.4906\\
			    \ \&$\mathcal{G}_{0,1}(t_{fin})$& $\widetilde{cor}_{sto}-\overline{cor} $ &\textbf{0.1381}&\textbf{0.1361}&	&\textbf{0.1343}&\textbf{0.1309}&	&\textbf{0.1370}&\textbf{0.1319}\\			
			   & $\widetilde{cor}_{exa}-\overline{cor} $ &\textbf{0.1455}&\textbf{0.1404}&	&\textbf{0.1343}&\textbf{0.1331}&	&\textbf{0.1369}&\textbf{0.1246}\\ 
			    & $\widehat{cor}-\overline{cor} $ &-0.0022&-0.0032& &-0.0022&-0.0099&	&-0.0026&-0.0148\\
			
			$\mathcal{G}_{0,1}(t_{int})$&$\overline{cor} $&0.6494&0.6566&	&0.6490&0.6591&	&0.6474&0.6603\\ 
			    \ \&$\mathcal{G}_{0,0}(t_{fin})$& $\widetilde{cor}_{sto}-\overline{cor} $ &-0.0073&-0.0137&	&-0.0074&-0.0145&	&-0.0035&-0.0130\\
			    & $\widetilde{cor}_{exa}-\overline{cor} $ &-0.0020&-0.0097&	&-0.0067&-0.0112&	&-0.0027&-0.0151\\
			    & $\widehat{cor}-\overline{cor} $ &-0.0021&-0.0054&	&-0.0034&-0.0081&	&-0.0037&-0.0096\\             
			
			$\mathcal{G}_{0,0}(t_{int})$&$\overline{cor} $&0.4172&0.4094&	&0.4212&0.4128&	&0.4215&0.4128\\
			    \ \&$\mathcal{G}_{0,1}(t_{fin})$& $\widetilde{cor}_{sto}-\overline{cor} $ &\textbf{0.1108}&\textbf{0.1041}&	&\textbf{0.1092}&\textbf{0.1019}&	&\textbf{0.1158}&\textbf{0.1047}\\
			    & $\widetilde{cor}_{exa}-\overline{cor} $ &\textbf{0.1182}&\textbf{0.1090}&	&\textbf{0.1105}&\textbf{0.1051}&	&\textbf{0.1170}&\textbf{0.1001}\\
			    & $\widehat{cor}-\overline{cor} $ &-0.0031&-0.0069&	&-0.0024&-0.0106&	&0.0005&-0.0132\\
			\hline
		\end{tabular}
	\end{minipage}
	\vspace{5pt}
\end{table}
%\end{sidewaystable}
%%%%  end Supplemental table 5  %%%%

  %%%% Supplemental table 6  %%%%
 %\begin{sidewaystable}
 \begin{table}
 	\begin{minipage}{160mm}\centering
 		\caption{Comparison of the correlations computed using different methods: the correlations calculated directly from the simulated samples ($\overline{cor}$), the predicted values using either stochastic process ($\widetilde{cor}_{sto}$) or exact distribution ($\widetilde{cor}_{exa}$), and the data-driven estimation ($\widehat{cor}$). The sample correlations were treated as the gold standard for comparison of other methods. In comparison with the gold-standard mean, correlations with difference $5-10\%$ were made \textit{italic}, and $>10\%$ were made \textbf{bold}. The simulations in this table include \emph{violations I (accrual), II (censoring), and IV(delayed time)}.  }
 		\label{tab:corr_all3}
		\begin{tabular}{clcclcclcc}\hline\hline
	{Correlation }&\phantom{}&\multicolumn{2}{c}{ $\theta=0.7$} &
	&\multicolumn{2}{c}{ $\theta=0.6$} &\phantom{}&\multicolumn{2}{c}{ $\theta=0.5$}\\ [-1pt]\cline{3-4} \cline{6-7} \cline{9-10}\\[-10pt]
	Pair& &$H_0$&$H_1$& &$H_0$&$H_1$& &$H_0$&$H_1$ \\ \hline
 			$\mathcal{G}_{0,1}(t_{int})$&$\overline{cor} $&0.8267&0.8288&	&0.8261&0.8284&	&0.8248&0.8297\\						
 			    \ \&$\mathcal{G}_{0,0}(t_{int})$& $\widetilde{cor}_{sto}-\overline{cor} $ &0.0036&0.0020&	&0.0040&0.0025&	&0.0051&0.0016\\						
 			    & $\widetilde{cor}_{exa}-\overline{cor} $ &0.0056&0.0042&	&0.0059&0.0048&	&0.0070&0.0040\\						
 			    & $\widehat{cor}-\overline{cor} $ &-0.0009&-0.0007&	&-0.0007&-0.0002&	&-0.0001&-0.0015\\
 			
 			$\mathcal{G}_{0,1}(t_{fin})$&$\overline{cor} $&0.8508&0.8567&	&0.8482&0.8569&	&0.8452&0.8579\\						
 			   \ \&$\mathcal{G}_{0,0}(t_{fin})$& $\widetilde{cor}_{sto}-\overline{cor} $ &0.0189&0.0208&	&0.0176&0.0208&	&0.0163&0.0194\\						
 			    & $\widetilde{cor}_{exa}-\overline{cor} $ &0.0201&0.0223&	&0.0188&0.0225&	&0.0176&0.0214\\
 			    & $\widehat{cor}-\overline{cor} $ &-0.0010&-0.0042&	&-0.0008&-0.0054&	&-0.0002&-0.0074\\
 			
 			$\mathcal{G}_{0,0}(t_{int})$&$\overline{cor} $&0.7772&0.7776&	&0.7763&0.7774&	&0.7757&0.7778\\			
 			   \ \&$\mathcal{G}_{0,0}(t_{fin})$& $\widetilde{cor}_{sto}-\overline{cor} $ &-0.0039&-0.0037&	&-0.0035&-0.0016&	&0.0002&0.0007\\
 			   & $\widetilde{cor}_{exa}-\overline{cor} $ &0.0006&-0.0009&	&-0.0043&0.0002&	&-0.0007&-0.0039\\			
 			    & $\widehat{cor}-\overline{cor} $ &-0.0027&-0.0030&	&-0.0017&-0.0028&	&-0.0011&-0.0032\\
 			
 			$\mathcal{G}_{0,1}(t_{int})$&$\overline{cor} $&0.6099&0.6076&	&0.6158&0.6209&	&0.6219&0.6310\\
 			    \ \&$\mathcal{G}_{0,1}(t_{fin})$& $\widetilde{cor}_{sto}-\overline{cor} $ &0.0260&0.0105& &0.0232&-0.0015&	&0.0255&-0.0085\\			
 			   & $\widetilde{cor}_{exa}-\overline{cor} $ &\textit{0.0334}&0.0148&	&0.0232&0.0007&	&0.0255&-0.0158\\ 
 			    & $\widehat{cor}-\overline{cor} $ &-0.0029&-0.0063&	&0.0000&-0.0112&	&0.0005&-0.0147\\
 			
 			$\mathcal{G}_{0,1}(t_{int})$&$\overline{cor} $&0.6436&0.6458&	&0.6414&0.6462&	&0.6413&0.6510\\ 
 			    \ \&$\mathcal{G}_{0,0}(t_{fin})$& $\widetilde{cor}_{sto}-\overline{cor} $ &-0.0014&-0.0028&	&0.0002&-0.0016&	&0.0025&-0.0038\\
 			    & $\widetilde{cor}_{exa}-\overline{cor} $ &0.0039&0.0012&	&0.0009&0.0017&	&0.0034&-0.0058\\
 			    & $\widehat{cor}-\overline{cor} $ &-0.0038&-0.0043&	&-0.0020&-0.0047& &-0.0025&-0.0095\\             
 			
 			$\mathcal{G}_{0,0}(t_{int})$&$\overline{cor} $&0.5044&0.5070&	&0.5093&0.5164&	&0.5117&0.5230\\
 			    \ \&$\mathcal{G}_{0,1}(t_{fin})$& $\widetilde{cor}_{sto}-\overline{cor} $ &0.0236&0.0065&	&0.0211&-0.0018&	&0.0255&-0.0056\\
 			    & $\widetilde{cor}_{exa}-\overline{cor} $ &\textit{0.0311}&0.0114&	&0.0223&0.0015&	&\textit{0.0268}&-0.0102\\
 			    & $\widehat{cor}-\overline{cor} $ &-0.0031&-0.0090&	&-0.0011&-0.0115&	&0.0015&-0.0126\\
 			\hline
 		\end{tabular}
 	\end{minipage}
 	\vspace{5pt}
 \end{table}
 %\end{sidewaystable}
 %%%%  end Supplemental table 6  %%%%

\end{document}
